# Supplementary material for: SNIP: Bridging Mathematical Symbolic and Numeric Realms with Unified Pre-training
Source: arXiv:2310.02227 source file (2024-03-15)
Supplement: Supplementary file 1 [file tab_discussion_appendix.tex]

\begin{wraptable}[10]{r}{0.7\linewidth}
% \begin{table}[!ht]
    \centering
    \vspace{-1.0em}

    \caption{Some potential applications of \modelname are categorized based on the input, output, and guiding (informing) modalities.}
    \label{tab:discussion_appendix}
    {\fontsize{35}{35}\selectfont
    \resizebox{\linewidth}{!}{
    \begin{tabular}{llll}
    \toprule
        \textbf{Input Modality} & \textbf{Output Modality} & \textbf{Guiding Modality} & \textbf{Potential Tasks}  \\
    \midrule
      Symbolic   &  Symbolic &  Numeric & Symbolic Integration/Derivation, Solving Differential Equations  \\
     Symbolic    &  Numeric & Numeric & Solving and Predicting Ordinary or Partial Differential Equations \\
    Symbolic     &  Numeric Properties & Numeric &  Optimization, Convexity, Numeric Trends, etc. \\
      Numeric   &  Symbolic & Symbolic &  Symbolic Regression, System Identification \\
      Numeric   &  Numeric & Symbolic &  Zero-shot Super-resolution, Extrapolation, Time-series Forecasting \\
     Numeric   &  Symbolic Properties & Symbolic &  Expression Classification \\
     \bottomrule
    \end{tabular}
    }
    }
    \label{tab:potential-app}
% \end{table}
\end{wraptable}
